# Supplementary material for: A Note on Hyperbolic Relaxation of the Navier-Stokes-Cahn-Hilliard system for incompressible two-phase flow
Source: arXiv:2412.11904 source file (2024-12-17)
Supplement: Supplementary file 1 [file Appendix.tex]

In order to find out the eigenvalues, roots of \eqref{charactpolynomial} should be found. Factorization of term in \eqref{testcase1} is not easy to write each root for all state space explicitly. Therefore, we find the roots  for one state space, which is $u=0$. It gives 

\begin{equation}\label{charac.polynomialu0}
    p(\lambda) = \lambda^4  - 
    \left(\left(W''(c^{\varepsilon}) + \frac1{\beta} \right) \left(\frac1{\delta^2} - c^2\right) + \frac1{\alpha}\right) \lambda^2  \\ +
     + \dfrac{1}{\alpha \delta^2}\left(W''(c^{\varepsilon}) + \frac1\beta \right).
\end{equation}

To have four roots we write fourth degree polynomial two quadratic polynomials such that
\begin{equation}\label{generalquadraticform}
    (\lambda^2 + a\lambda + b) (\lambda^2 + f\lambda + d)
\end{equation}
By using \eqref{charac.polynomialu0}, we can find $a,b,f$ and $d$. There are three steps, which are 
\begin{enumerate}
    \item $f+a = 0$
    \item $d + af + b = - \left(W''(c) + \frac1 \beta \right) \left(\frac1 \delta^2 + c^2 \right) - \dfrac1 \alpha $
    \item $bd$ = $\dfrac{1}{\alpha \beta^2} \left(W''(c) + \frac1 \beta \right)$
\end{enumerate}

The first step gives $f=-a$.
The third step gives $b = - \frac1 {\alpha}$ and $d = - \dfrac{1}{\beta^2} \left(W''(c) + \frac1 \beta \right)$. 
Now we can go to the second step and we obtain 
\begin{equation*}
    af = - c^2 \left(W''(c) + \frac1 \beta \right) \to f = \pm \sqrt{c^2 \left(W''(c) + \frac1 \beta \right)} 
\end{equation*}
We choose $f= \sqrt{c^2 \left(W''(c) + \frac1 \beta \right)} $, so $a = - \sqrt{c^2 \left(W''(c) + \frac1 \beta \right)}$. 
Then we can rewrite the \eqref{charac.polynomialu0} with $a,b,f,d$ as following
\begin{equation}\label{character.polynofor_factorization}
    (\lambda^2 - \sqrt{c^2 \left(W''(c) + \frac1 \beta \right)} \lambda - \frac1 {\alpha} ) (\lambda^2 + \sqrt{c^2 \left(W''(c) + \frac1 \beta \right)}\lambda + - \dfrac{1}{\beta^2} \left(W''(c) + \frac1 \beta \right)) = 0
\end{equation}
Next step we should compute the discriminant of the each quadratic formula and find $\lambda$ which has been shown in \eqref{eigenvalues}.
